# Supplementary material for: Non-Equilibrium Phonon Transport Across Nanoscale Interfaces
Source: arXiv:1811.01059 source file (2018-11-02)
Supplement: Supplementary file 1 [file supplementary.pdf]

# Supplemental Matierial for : Non-Equilibrium Phonon Transport Across Nanoscale Interfaces


Georgios Varnavides,[1,2,3] Adam S. Jermyn,[4,5] Polina Anikeeva,[1,2] and Prineha Narang[3]

[1]Department of Materials Science and Engineering, Massachusetts Institute of Technology, Cambridge, MA, USA

[2]Research Laboratory of Electronics, Massachusetts Institute of Technology, Cambridge, MA, USA

[3]John A. Paulson School of Engineering and Applied Sciences, Harvard University, Cambridge, MA,USA

[4]Kavli Institute for Theoretical Physics, University of California at Santa Barbara, Santa Barbara, CA 93106, USA

[5]Institute of Astronomy, University of Cambridge, Madingley Rd, Cambridge CB3 0HA, UK



(Dated: November 2, 2018)


## 1. RECURSIVE SOLUTION TO BOLTZMANN TRANSPORT EQUATION

We derive the recursive solution to a general ballistic transport problem with linear collision and a source term. This is governed by the differential equation

$$\sum_j \left(\frac{D}{Dt}\right)_{ij} \phi_j = S_i^{(0)} - \sum_j C_{ij}\phi_j, \tag{1}$$

where $S^{(0)}$ is the initial source term, $C$ is the collision matrix, and $\phi$ is the vector density of states whose evolution we'd like to track. The differential operator $D/Dt$ is defined as

$$\left(\frac{D}{Dt}\right) = \left(\frac{\partial}{\partial t} + \sum_k v_{ik}\nabla_k\right)\delta_{ij}, \tag{2}$$

where $v$ is the ballistic velocity operator, and $\nabla$ is the *nabla* operator. In steady state, $\partial/\partial t \to 0$, and eq. (1) reduces to

$$\sum_k v_{ik}\nabla_k\phi_i = S_i^{(0)} - \sum_j C_{ij}\phi_j \tag{3}$$

This can be re-written in the form

$$\sum_j \left(\delta_{ij}\sum_k v_{ik}\nabla_k + C_{ij}\right)\phi_j = S_i^{(0)}, \tag{4}$$

which highlights that, for a given discretization of space, the solution $\phi$ may be obtained via a matrix inversion. The matrix to be inverted however, exists over the joint space of spatial and state dimensions, so instead - we proceed iteratively. We first split $C$ into diagonal and off-diagonal terms

$$C_{ij} = \tau_i^{-1}\delta_{ij} + M_{ij}, \tag{5}$$

where $\tau_i$ is the lifetime of the carrier in state $i$. We may thereby express eq. (4) as

$$\sum_j \left(\delta_{ij}\sum_k v_{ik}\nabla_k + \delta_{ij}\tau_i^{-1}\right)\phi_j = S_i^{(0)} + \sum_j M_{ij}\phi_j, \tag{6}$$

where the operator which acts on $\phi$ on the left-hand side is diagonal in state space, and the operator which acts on it on the right hand side is diagonal in position space.

Let $G_i$ be the Green's function which inverts this operator. Our iteration scheme then amounts to the following:

$$\phi_i^{(n)} = G_i\left(S_i^{(n)}\right) \tag{7a}$$

$$S_i^{(n+1)} = -\sum_j M_{ij}\phi_j^{(n)} \tag{7b}$$

Where $\phi_i^{(n)}$ depends on the $n^{th}$ power of G, and is defined as

$$\phi_i = \sum_{n=0}^{\infty}\phi_i^{(n)} \tag{8}$$

Equations (7a) and (7b) may be written in a form similar to the *Jacobi iterative method*

$$\phi^{(n)} = -GM\phi^{(n-1)} \tag{9}$$

where all summation indices have been dropped for clarity. The iterative scheme converges if and only if the spectral radius of $GM$ is less than unity. This is not guaranteed *a priori*, so the scheme could fail. To remedy this, we switch to a *weighted Jacobi* scheme

$$\phi^{(n)} = -\omega GM\phi^{(n-1)} + (1-\omega)\phi^{(n-1)} \tag{10a}$$

$$\phi^{(0)} = \omega GS^{(0)} \tag{10b}$$

where $\omega \in (0,1)$ is the weight parameter, chosen so that the spectral radius of $\omega GM$ is less than unity. This is guaranteed to converge as long as the matrix $G^{-1} - M$ is diagonally dominant.

Because the joint position-state space over which $GM$ is defined is extremely large we cannot explicitly construct this operator and hence cannot directly use its spectral radius to motivate a choice of $\omega$. However the Green's function acting on a spatially homogeneous system reduces to $\tau_i\delta_{ij}$, so we may use the operator $\tau M$ to estimate the spectral radius of $GM$. Furthermore, in the following section we show that the collision matrix $C$ is indeed strictly diag-

onally dominant, so at least in the spatially homogeneous case $G^{-1} - M = -C$ is diagonally dominant, motivating this scheme.

A number of observations in the *Letter* rely on the exact scattering history which is only strictly equal to $\phi^{(n)}$ for a choice of $\omega = 1$. To address this, we reconstruct the scattering history *a posteriori*. Let the iteration matrix $Q = -GM$ and note that eq. (10a) can be written as

$$\phi^{(n)} = \sum_{j=0}^{n} (\omega Q)^j (1-\omega)^{n-j} \binom{n}{j} \phi^{(0)} \tag{11}$$

Since $Q$ is the operator which scatters and propagates carriers, we can define the population of carriers following $k$ scattering events, $\psi_k$ as those that arrive via $k$ applications of $Q$.

$$\psi_k = \sum_{n=k}^{\infty} \omega^k (1-\omega)^{n-k} \binom{n}{k} Q^k \phi^{(0)} \tag{12}$$

In order to calculate $\psi_k$, we need access to $Q^k \phi^{(0)}$. This can be accomplished by separating eq. (11)

$$\phi^{(n)} = \sum_j Z_{nj} Q^j \phi^{(0)} \tag{13a}$$

to a purely combinatorial component

$$Z_{nj} = \omega^j (1-\omega)^{n-j} \binom{n}{j}, \tag{13b}$$

to finally obtain

$$Q^k \phi^{(0)} = \sum_l Z^{-1}_{jl} \phi^{(n)} \tag{14}$$

With eq. (14) it is possible to compute $\psi_k$ and thus reconstruct the full scattering history as a post-processing step. This is guaranteed to be possible, since $Z$ is non-singular.

## 2. ANHARMONIC SCATTERING PROCESSES

The phonon Boltzmann Transport Equation requires phonon group velocities, and the scattering matrix as material inputs. In this section, we summarize the rate expressions for the scattering processes we consider in bulk. All first principles calculations were performed using Quantum Espresso [1, 2], based on density functional theory (DFT). In particular third-order interatomic force constants and anharmonic scattering rates were computed using the d3q and thermal2 suite of codes [3–8].

We consider two types of anharmonic scattering processes inside bulk materials, namely three-phonon scattering and phonon-isotope scattering. The intrinsic three-phonon scattering can be further separated into 'coalescence processes"(+) and 'decay processes"(−) whose rates are given by [5, 9]

$$\begin{aligned} P^{\pm}_{\boldsymbol{q}s,\boldsymbol{q}'s',\boldsymbol{q}''s''} &= 2\pi \bar{n}_{\boldsymbol{q}s} \left( \bar{n}_{\boldsymbol{q}'s'} + \frac{1}{2} \mp \frac{1}{2} \right) (\bar{n}_{\boldsymbol{q}''s''} + 1) \\ &\times \left| V_3\left(-\boldsymbol{q}s, \mp \boldsymbol{q}'s', \boldsymbol{q}''s''\right)\right|^2 \delta(\omega_{\boldsymbol{q}s} \pm \omega_{\boldsymbol{q}'s'} - \omega_{\boldsymbol{q}''s''}) \end{aligned} \tag{15}$$

$V_3\left(\boldsymbol{q}s, \boldsymbol{q}'s', \boldsymbol{q}''s''\right)$ is the anharmonic coupling given by

$$\begin{aligned} V_3\left(\boldsymbol{q}s, \boldsymbol{q}'s', \boldsymbol{q}''s''\right) &= \left( \frac{\hbar}{8N\omega_{\boldsymbol{q}s}\omega_{\boldsymbol{q}'s'}\omega_{\boldsymbol{q}''s''}} \right)^{1/2} \\ &\times \sum_{bb'b''} \sum_{\alpha\beta\gamma} \tilde{\Psi}_{\alpha\beta\gamma}\left(\boldsymbol{q}b, \boldsymbol{q}'b', \boldsymbol{q}''b''\right) (m_b m_{b'} m_{b''})^{-1/2} \\ &\times e_\alpha(b|\boldsymbol{q}s) e_\beta(b'|\boldsymbol{q}'s') e_\gamma(b''|\boldsymbol{q}''s''), \end{aligned}$$

$\boldsymbol{e}(b|\boldsymbol{q}s)$ is the eigenvector of the $b^{th}$ atom in mode $\boldsymbol{q}s$, $m$ are atomic masses, $N$ is the number of q-points, and greek letters denote cartesian directions. $\tilde{\Psi}\left(\boldsymbol{q}b, \boldsymbol{q}'b', \boldsymbol{q}''b''\right)$ is the Fourier transformed third-order interatomic force constants tensor given by

$$\tilde{\Psi}\left(\boldsymbol{q}b, \boldsymbol{q}'b', \boldsymbol{q}''b''\right) = \sum_{l'l''} \Psi\left(0b, l'b', l''b''\right) e^{i\left(q'l' + q''l''\right)},$$

where $l$ is a supercell index, and all other symbols are as previously defined in the *Letter*.

Similarly, the rate for a phonon-isotope event is [5]

$$\begin{aligned} P^{isot}_{\boldsymbol{q}s,\boldsymbol{q}'s'} &= \frac{\pi}{2N} \left( \bar{n}_{\boldsymbol{q}s} \bar{n}_{\boldsymbol{q}'s'} + \frac{\bar{n}_{\boldsymbol{q}s} + \bar{n}_{\boldsymbol{q}'s'}}{2} \right) \omega_{\boldsymbol{q}s} \omega_{\boldsymbol{q}'s'} \\ &\times \sum_b g_b \left| \sum_\alpha e_\alpha(b|\boldsymbol{q}s)^* \cdot e_\alpha(b|\boldsymbol{q}'s') \right|^2 \delta(\omega_{\boldsymbol{q}s} - \omega_{\boldsymbol{q}'s'}), \end{aligned} \tag{16}$$

where

$$g_b = \frac{(m_b - \langle m_b \rangle)^2}{\langle m_b \rangle^2} \tag{7}$$

is the mass average of atom $b$.

Combining eqs. (15) and (16), the total anharmonic scattering matrix inside bulk materials is given by [5, 10]

$$\begin{aligned} A_{\mu,\mu'} &= \left[ \sum_{\mu'',\mu'''} \left( P^+_{\mu,\mu''',\mu''} + \frac{P^+_{\mu'',\mu''',\mu}}{2} \right) + \sum_{\mu''} P^{isot}_{\mu,\mu''} \right] \delta_{\mu,\mu'} \\ &- \sum_{\mu''} \left( P^-_{\mu,\mu'',\mu'} - P^-_{\mu,\mu',\mu''} + P^-_{\mu',\mu'',\mu} \right) + P^{isot}_{\mu,\mu'}, \end{aligned} \tag{17}$$

where we've switched to the compact mode index $\mu$, as in the *Letter*.

It can be shown that the scattering matrix is symmetric and positive semidefinite [5]. This is a stricter condition than our required strictly diagonally dominant condition,

and thus the iterative scheme described in the previous section is guaranteed to converge for appropriate choices of weight $\omega$ as long as the spatial degrees of freedom do not amplify the spectral radius of the system. This is unlikely to emerge, as a spatially varying system with even partially-absorbing boundary conditions loses carriers more readily than an infinite homogeneous one, though the possibility remains that under certain conditions our scheme could become ill-conditioned.

## 3. INTERFACIAL STRAIN COUPLING

In this section, we start with eq. (8) of the *Letter*, i.e. the perturbation Hamiltonian describing phonon-strain coupling, and derive the scattering rates following Carruthers [11, 12].

$$H' = \frac{\hbar}{4\rho\Omega} c_2(\mu_1, \mu_2) \prod_{i=1}^{2} \left( a^\dagger_{\mu_i} + a_{\mu_{-i}} \right) \tag{18}$$

Recall that the process involves two phonons (as evidenced by the product of two pairs of creation/annihilation operators), coupling with the external strain field via

$$\begin{aligned} c_2\left(\boldsymbol{q}s, \boldsymbol{q}'s'\right) &= \sum_{bb'b''} \sum_{\alpha\beta\gamma} \tilde{\Psi}_{\alpha\beta\gamma}\left(\boldsymbol{q}b, \boldsymbol{q}'b', (\boldsymbol{q}' - \boldsymbol{q})b''\right) \\ &\times \frac{e_\alpha(b|\boldsymbol{q}s)}{\sqrt{\omega_{\boldsymbol{q}s} m_b}} \frac{e_\beta(b'|\boldsymbol{q}'s')}{\sqrt{\omega_{\boldsymbol{q}'s'} m_{b'}}} v_\gamma(\boldsymbol{q}' - \boldsymbol{q}), \end{aligned} \tag{19}$$

where the excess momentum is evalutated at the Fourier transformed external strain field $\boldsymbol{v}(\boldsymbol{q}' - \boldsymbol{q})$.

Using eqs. (18) and (19), the scattering rate is therefore given by

$$\begin{aligned} P^{strain}_{\boldsymbol{q}s,\boldsymbol{q}'s'} &= \frac{\pi}{8\rho^2\Omega^2} \left( \bar{n}_{\boldsymbol{q}s}\bar{n}_{\boldsymbol{q}'s'} + \frac{\bar{n}_{\boldsymbol{q}s} + \bar{n}_{\boldsymbol{q}'s'}}{2} \right) \\ &\times \left| c_2\left(\boldsymbol{q}s, \boldsymbol{q}'s'\right) \right|^2 \delta(\omega_{\boldsymbol{q}s} - \omega_{\boldsymbol{q}'s'}) \end{aligned} \tag{20}$$

We note that $\hbar s$ cancels out, making the result fully classical.

We now turn to deriving the external strain for the specific case of a semi-coherent interface. In particular, we look at the dilatation caused by misfit dislocations. The displacement fields for a sinlge edge dislocation are readily provided by Linear elasticity as [13]

$$\begin{aligned} u_x &= \frac{b}{2\pi}\left[\theta + \frac{\sin(2\theta)}{4(1-\nu)}\right] \\ u_y &= -\frac{b}{2\pi}\left[\frac{(1-2\nu)}{2(1-\nu)}\log\left(\frac{r_0}{r}\right) + \frac{\cos(2\theta)}{4(1-\nu)}\right] \\ u_z &= 0, \end{aligned} \tag{21}$$

where $b$ is the magnitude of the dislocation Burger's vector, $\nu$ is the material's Poisson ratio, $r_0$ is the dislocation core radius, and $r, \theta$ are polar coordinates. The dilatation of eq. (21) for the usual approximation of $r_0 \approx b$ is

$$\begin{aligned} \Delta(r) = \nabla\cdot\left\{u_x, u_y, u_z\right\} &= -\frac{b}{2\pi}\left[\frac{1-2\nu}{2(1-\nu)}\frac{\sin\theta}{r}\right] \\ \Delta(x,y) &= -\frac{b}{2\pi}\left[\frac{1-2\nu}{2(1-\nu)}\frac{y}{x^2+y^2}\right] \end{aligned} \tag{22}$$

Working under the assumption of linear elasticity, we can express the additive dilatation of an infinite array of edge dislocations with a period $d$ as

$$\begin{aligned} \Delta^\infty(x,y) &= -\frac{b}{2\pi}\left[\frac{1-2\nu}{2(1-\nu)}\right]\sum_{n=-\infty}^{\infty}\frac{y}{(x-nd)^2+y^2} \\ &= -\frac{b}{2\pi}\left[\frac{1-2\nu}{2(1-\nu)}\right]\frac{\sinh(2\pi y/d)}{\cosh(2\pi y/d)-\cos(2\pi x/d)} \end{aligned} \tag{23}$$

Where we note that the result is (naturally) periodic along the interface. The dilatational field is plotted in Fig. 3c of the *Letter*.We can take the Fourier transform of eq. (23) by the following change of variables: $\alpha = 2\pi x/d, \beta = 2\pi y/d$, $k_x = q_x d/2\pi$, and $k_y = q_y d/2\pi$ to give

$$\Delta^\infty(q) = -\frac{b}{\Omega^{2/3}}\left[\frac{1-2\nu}{(1-\nu)}\right]\frac{iq_y}{(q_x^2+q_y^2)} \tag{24}$$

Where the $\Omega^{2/3}$ factor was accumulated as consequence of integrating along the interface. We can supplement eq. (24) with an additional factor of $\Delta(q_z)$ resulting from integrating out of plane, to obtain [12]

$$\boldsymbol{v}(\boldsymbol{q}) = \frac{b}{\Omega^{2/3}}\left[\frac{1-2\nu}{(1-\nu)}\right]\frac{q_y}{(q_x^4+2q_x^2q_y^2+q_y^4)}\Delta(q_z)\boldsymbol{q} \tag{25}$$

Finally, we note the natural result that $\boldsymbol{v}(\boldsymbol{q})$ is parallel to $\boldsymbol{q}$ since the field's rotation, $R = \nabla\times\left\{u_x, u_y, u_z\right\}$, is zero.


[1] P. Giannozzi, S. Baroni, N. Bonini, M. Calandra, R. Car, C. Cavazzoni, D. Ceresoli, G. L. Chiarotti, M. Cococcioni, I. Dabo, A. D. Corso, S. de Gironcoli, S. Fabris, G. Fratesi, R. Gebauer, U. Gerstmann, C. Gougoussis, A. Kokalj, M. Lazzeri, L. Martin-Samos, N. Marzari, F. Mauri, R. Mazzarello, S. Paolini, A. Pasquarello, L. Paulatto, C. Sbraccia, S. Scandolo, G. Sclauzero, A. P. Seitsonen, A. Smogunov, P. Umari, and R. M. Wentzcovitch, Journal of Physics: Condensed Matter **21**, 395502 (2009).

[2] P. Giannozzi, O. Andreussi, T. Brumme, O. Bunau, M. B. Nardelli, M. Calandra, R. Car, C. Cavazzoni, D. Ceresoli, M. Cococcioni, N. Colonna, I. Carnimeo, A. D. Corso, S. de Gironcoli, P. Delugas, R. A. DiStasio, A. Ferretti, A. Floris, G. Fratesi, G. Fugallo, R. Gebauer, U. Gerst-

mann, F. Giustino, T. Gorni, J. Jia, M. Kawamura, H.-Y. Ko, A. Kokalj, E. Küçükbenli, M. Lazzeri, M. Marsili, N. Marzari, F. Mauri, N. L. Nguyen, H.-V. Nguyen, A. O. de-la Roza, L. Paulatto, S. Poncé, D. Rocca, R. Sabatini, B. Santra, M. Schlipf, A. P. Seitsonen, A. Smogunov, I. Timrov, T. Thonhauser, P. Umari, N. Vast, X. Wu, and S. Baroni, Journal of Physics: Condensed Matter **29**, 465901 (2017).

[3] M. Lazzeri and S. de Gironcoli, Physical Review Letters **81**, 2096 (1998).

[4] L. Paulatto, F. Mauri, and M. Lazzeri, Physical Review B **87** (2013), 10.1103/physrevb.87.214303.

[5] G. Fugallo, M. Lazzeri, L. Paulatto, and F. Mauri, Physical Review B **88** (2013), 10.1103/physrevb.88.045430.

[6] G. Fugallo, A. Cepellotti, L. Paulatto, M. Lazzeri, N. Marzari, and F. Mauri, Nano Letters **14**, 6109 (2014).

[7] A. Cepellotti, G. Fugallo, L. Paulatto, M. Lazzeri, F. Mauri, and N. Marzari, Nature Communications **6** (2015), 10.1038/ncomms7400.

[8] L. Paulatto, I. Errea, M. Calandra, and F. Mauri, Physical Review B **91** (2015), 10.1103/physrevb.91.054304.

[9] S. L. Shindé and G. P. Srivastava, eds., *Length-Scale Dependent Phonon Interactions* (Springer New York, 2014).

[10] G. Srivastava, *The Physics of Phonons* (CRC Press, 1990).

[11] P. Carruthers, Physical Review **114**, 995 (1959).

[12] P. Carruthers, Reviews of Modern Physics **33**, 92 (1961).

[13] J. H. Weertman, *Dislocation Based Fracture Mechanics* (World Scientific Pub Co Inc, 1996).
